# Supplementary material for: Effect of Electron-Phonon and Electron-Impurity Scattering on Electronic Transport Properties of Silicon/Germanium Superlattices
Source: arXiv:2111.12831 source file (2021-11-24)
Supplement: Supplementary file 1 [file SM-Electron_Relaxation_in_Semiconductor_Superlattices.pdf]

# Effect of Electron-Phonon and Electron-Impurity Scattering on Electronic Transport Properties of Silicon/Germanium Superlattices

Manoj Settipalli, Vitaly S Proshchenko, and Sanghamitra Neogi*

*Ann and H.J. Smead Aerospace Engineering Sciences, University of Colorado Boulder, Boulder, Colorado 80303, USA*

E-mail: sanghamitra.neogi@colorado.edu

## Supplemental Materials

**First-Principles Geometry Optimization Computational Details:** The lattice constants of bulk Si and bulk Ge are obtained by optimizing their 2-atom primitive cells and 8-atom conventional cells, using Broyden-Fletcher-Goldfarb-Shanno Quasi-Newton algorithm (BFGS). We use $12 \times 12 \times 12$ and $6 \times 6 \times 6$ $k$-point mesh to sample the Brillouin zone (BZ) of 2-atom and 8-atom cells, respectively. We set the pseudopotentials and the rest of the parameters to be the same as described in section '2.3 Computational Details' of the article. We find the lattice constants of Si and Ge to be $a_{Si} = 5.40$ Å and $a_{Ge} = 5.62$ Å, respectively. The calculated Si lattice constant is $\sim 0.5\%$ lower than the measured value of 5.43 Å and that of Ge is $\sim 0.8\%$ lower than the measured value of 5.67 Å.[1] We then calculate the cross-plane lattice constants of Si/Ge SLs grown on Si and Ge substrates, using the bulk lattice constants. We fix the in-plane lattice constants to the respective bulk lattice constants and relax the structure along the cross-plane direction, using the BFGS method. The resulting

cross-plane lattice constants of SLs grown on Si substrate are: $\{Si_1Ge_3, Si_2Ge_2, Si_3Ge_1\}$ = $\{5.66$ Å, 5.57 Å, 5.48 Å$\}$. We implement this approach to model the SL assumed to be grown on $Si_{0.5}Ge_{0.5}$ substrate as well. The cross-plane lattice constants of $Si_2Ge_2$ SLs grown on $Si_{0.5}Ge_{0.5}$ and Ge substrates are 5.49 Å and 5.41 Å, respectively. To optimize the geometry of the relaxed $Si_2Ge_2$ SL, we relax the SL using the BFGS method in all directions, which yields an in-plane lattice constant of 5.50 Å.

## Hybrid Functional Band Gap Calculations

We employ the Perdrew-Zunger (PZ) parametrization of the local-density approximation (LDA) to perform the NSCF calculations on dense grids. This approximation is known to severely underestimate the band gap of both Si and Ge. In particular, PZ-LDA predicts Ge to be metal-like with $\sim 0$ eV direct band gap, as opposed to the measured indirect band gap of 0.66 eV at $L$-point. On the other hand, band gap of Si is calculated to be around $\sim 0.6$ eV, as opposed to the indirect band gap of 1.12 eV at $\Delta$-point. Therefore, to get a better estimate of the electronic transport properties of the Si/Ge SLs, it is imperative to correctly account for their band gaps. Hybrid functionals, particularly HSE06, have been demonstrated to provide better predictions of Si and Ge band gaps compared to LDA. While electronic structure property calculations using HSE06 potentials is implemented in Quantum Espresso, structural relaxation component is not implemented. However, using LDA relaxed lattice constants for HSE06 calculations will lead to incorrect band gap results. To overcome this drawback, we use Vienna Ab initio Simulation Package (VASP) for HSE06 hybrid functional calculations, which allows for structural relaxation as well. In its original form, VASP does not allow to simulate the effects of epitaxial relaxation (i.e. constrained optimization). We modify the source code to enable relaxation of the SLs in the cross-plane direction only. The calculated values of HSE06 band gaps of bulk Si and Ge using PBE and PBEsol exchange correlation functionals are shown in Table 1. We find that PBE-HSE06 and PBESol-HSE06 approaches produce the indirect band gap of Si closely, with a difference of

Table 1: Band gap (eV) of 2-atom primitive cells of bulk Si and bulk Ge, obtained using HSE06 hybrid functionals (VASP). The measured band gap values are extracted from Ref.[2,3]

| System | PBE-HSE06 | | PBESol-HSE06 | | Exp. | |
|---|---|---|---|---|---|---|
| | D | ID | D | ID | D | ID |
| Si | 3.34 | 1.16 | 3.31 | 1.08 | 3.40 | 1.12 |
| Ge | 0.59 | 0.68 | 0.70 | 0.65 | 0.81 | 0.66 |

0.04 eV and -0.04 eV, respectively. For the case of Ge, the indirect gap is very well predicted by PBE-HSE06, however, the direct gap is smaller than the indirect gap, indicating Ge to be a direct gap material. On the other hand, PBESol-HSE06 predicts both direct and indirect band gaps and their band order of Ge very well. Therefore, we employ PBESol-HSE06 hybrid functionals for the Si/Ge SL HSE06 band gap corrections used in the main article.

## Band Structures and Im$\Sigma^{\text{el-ph}}$ of Strained $Si_2Ge_2$ SLs

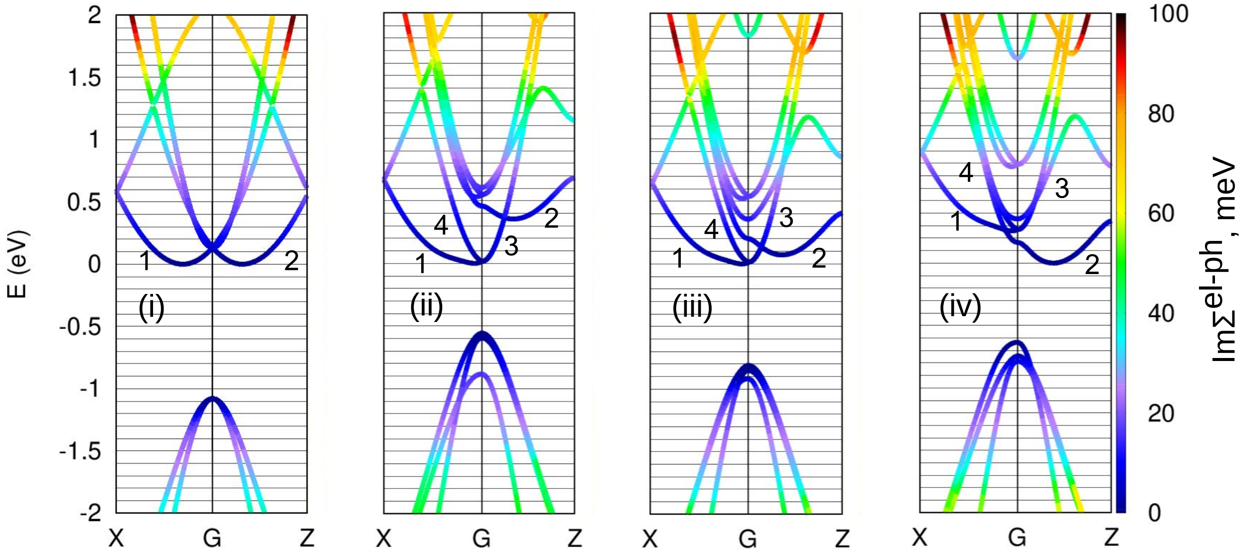


Figure 1: Electronic band structures and imaginary part of self-energies of (i) bulk Si and strained $Si_2Ge_2$ SLs with (ii) 0%, (iii) 1.85%, and (iv) 3.98% in-plane strains.

## Electron-Phonon Scattering Rate Convergence Tests

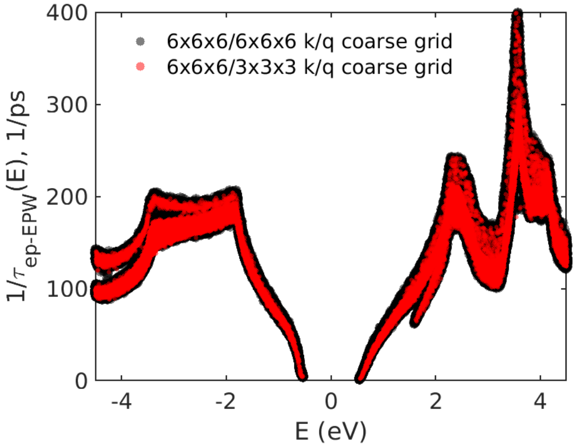


Figure 2: Results of convergence test of 8 atom bulk Si EPS rates. The EPS rates are computed from electron-phonon matrix elements. The matrix elements are obtained using different k/q coarse and fine grids. For both 6×6×6/6×6×6 and 6×6×6/3×3×3 k/q coarse grids, we interpolated results on 15,000/50,000 k/q fine grids.

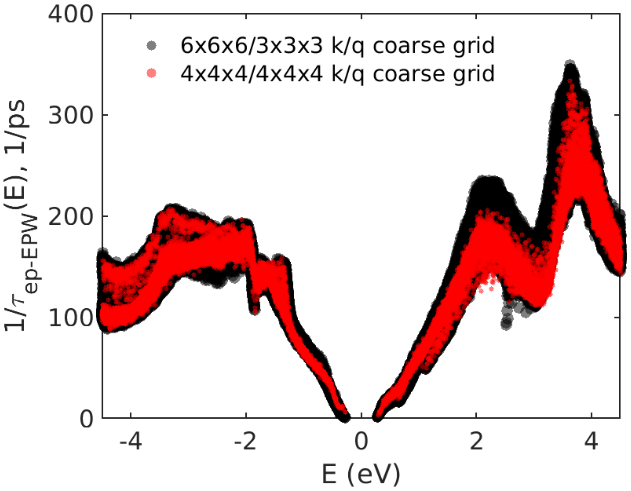


Figure 3: Results of convergence test of EPS rates of $Si_2Ge_2$ SL on Si substrate. The EPS rates are computed from electron-phonon matrix elements. The matrix elements are obtained using different k/q coarse and fine grids. We considered 15,000/50,000 (10,000/30,000) k/q fine grids for the 6×6×6/3×3×3 (4×4×4/4×4×4) k/q coarse grids, respectively. We use the coarse (fine) $4 \times 4 \times 4/4 \times 4 \times 4$ (10,000/30,000) BZ sampling to calculate all the Si/Ge SL EPS rates presented in the main article.

Note that we choose the red markers to be smaller than the black ones in Figs. 2 and 3, for better visual comparison. The rates overlap indicating grid size independence of results.

## Issues Related to the Determination of DOS Scattering Rates and Effect on Predicted Electronic Transport Properties

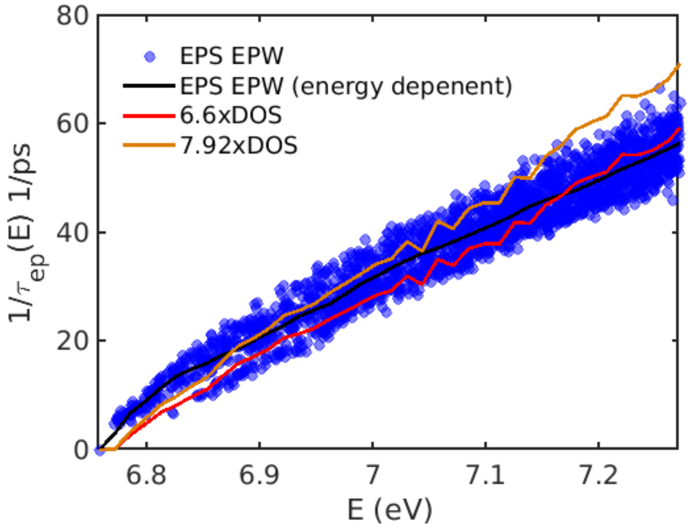


Figure 4: Determination of scaling factor, $K_{el-ph}$, to compute EPS rates in relaxed $Si_2Ge_2$ SL, using the DOS scattering approximation: $1/\tau_{\text{ep-DOS}}(E) = K_{\text{el-ph}} \times \text{DOS}(E)$. Blue circles represent electron-phonon scattering (EPS) rates predicted by the EPW approach. Black line represents the energy-averaged EPS rates ($1/\tau_{\text{ep-EPW}}(E)$), obtained using blue circles and Eq. 14 of the main article. Red and gold lines represent $1/\tau_{\text{ep-DOS}}(E)$ obtained with two different scaling factors, $K_{el-ph}$ =6.6 and 7.92, respectively. As can be seen, both the scaling factors could be used to describe $1/\tau_{\text{ep-DOS}}(E)$. However, they lead to different electronic transport properties.

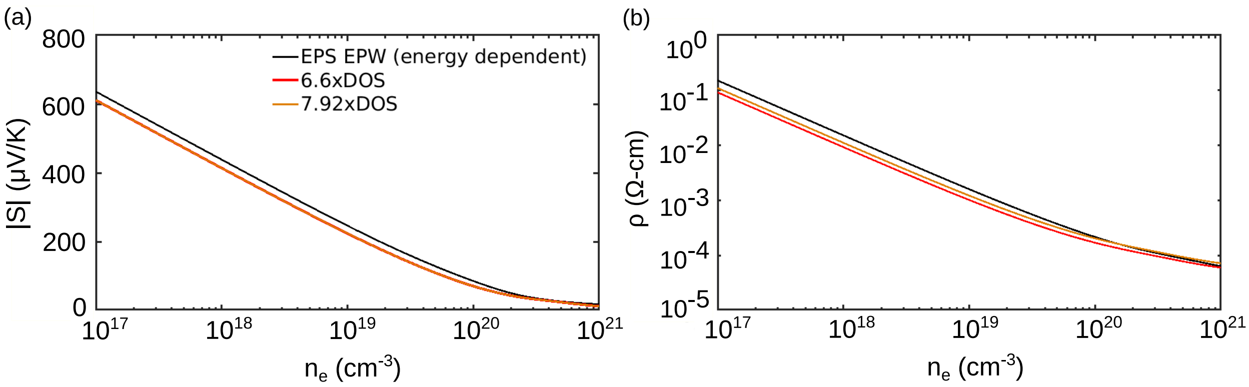


Figure 5: Comparison of predicted (a) S and (b) $\rho$ of relaxed $Si_2Ge_2$ SL, using EPS rates obtained with different approaches. Black lines show the predictions made using $\tau_{\text{ep-EPW}}(E)$. Red and gold lines show the predictions made using $\tau_{\text{ep-DOS}}(E)$, with $K_{el-ph}$ =6.6 and 7.92, respectively.

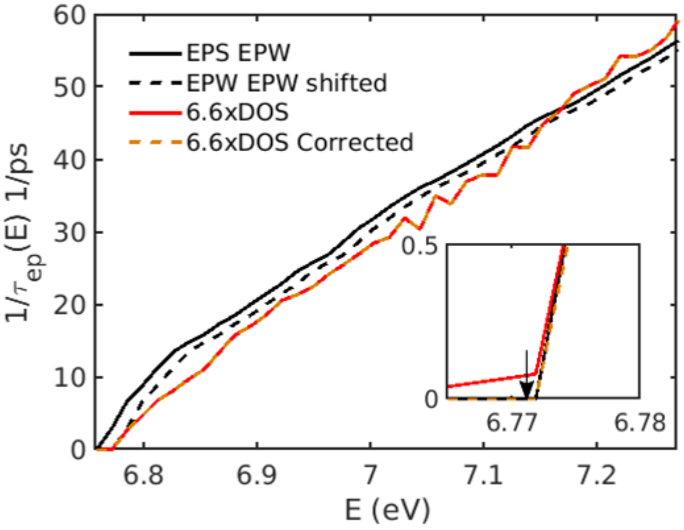


Figure 6: Different alignments of DOS(E) and $\tau_{\text{ep-EPW}}$(E) near the CBM for relaxed $Si_2Ge_2$ SL. Black solid line represents EPS rates predicted by EPW approach. Red solid line represents 6.6×DOS(E). The scaling factor is used for better visual comparison. The misalignment between the black and the red lines can be noted. We shift $\tau_{\text{ep-EPW}}$(E) to better align with DOS(E) (red). Black dashed line shows the shifted $1/\tau_{\text{ep-EPW}}$(E). Additionally, the small non-zero DOS(E) value near 6.77 eV is corrected to zero to get the corrected DOS(E) (gold dashed line) (see black arrow in inset). These adjustments are important while computing the BTE-integrals ($\mathcal{L}$) to predict S and $\rho$. The $\mathcal{L}$-integrands include the product of $\tau_{\text{ep-EPW}}$(E) and DOS(E).

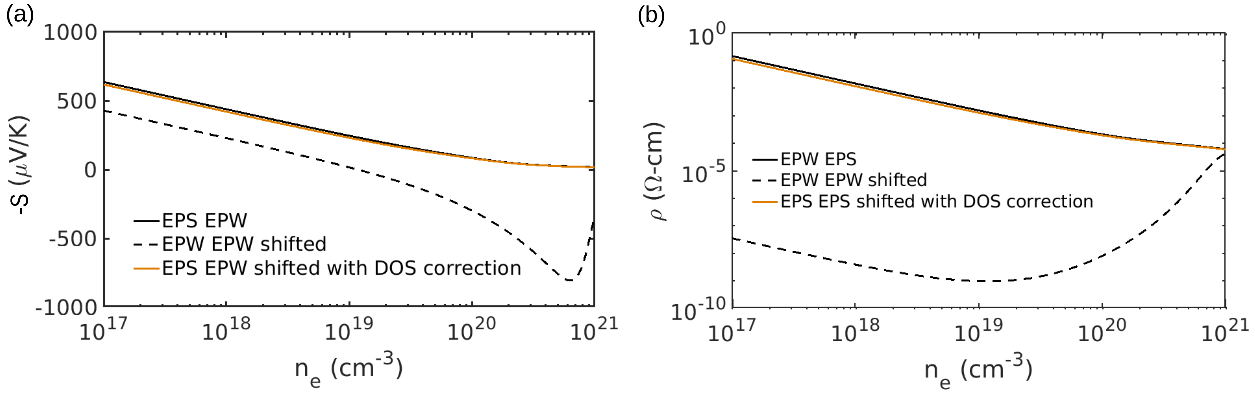


Figure 7: (a) S and (b) $\rho$ for relaxed $Si_2Ge_2$ SL obtained with $\tau_{\text{ep-EPW}}$(E) and DOS(E) values as shown in SI Fig. 6. Solid black line shows predictions obtained using $\tau_{\text{ep-EPW}}$(E) (solid black line in SI Fig. 6) and DOS(E). Dashed black line shows predictions obtained using shifted $\tau_{\text{ep-EPW}}$(E) (dashed black line in SI Fig. 6) and DOS(E). Solid gold line shows predictions obtained using shifted $\tau_{\text{ep-EPW}}$(E) (dashed black line in SI Fig. 6) and corrected DOS(E) (represented by the dashed gold line in SI Fig. 6).

Due to the fact that EPS rates and DOS are calculated using two different packages, EPW and Boltztrap, respectively, we aligned the DOS with the EPS scatter plots by aligning the first non-zero value of the DOS and EPS rates in the CB region. However, due to numerical inaccuracy, there can by a negligibly small finite DOS value in the region just below the CB edge, where DOS should be zero. This can lead to misalignment of the DOS with respect to EPS rates as shown in Fig. 6. In such cases, it is necessary to set the negligibly small finite DOS value below the CB edge to zero and re-align the EPS rates with the corrected DOS in-order to get meaningful resistivity predictions, as shown in Fig. 7. Shifting to EPS alone without correcting the DOS near CB edge can result in erroneous results as shown in Fig. 7 with dotted black lines. This is due to the fact that EPS is zero (or numerically set to a very small value) at the CBM while DOS is non-zero at this energy, albeit negligibly small.

## Group Velocity Squared of Strained $Si_2Ge_2$ SLs

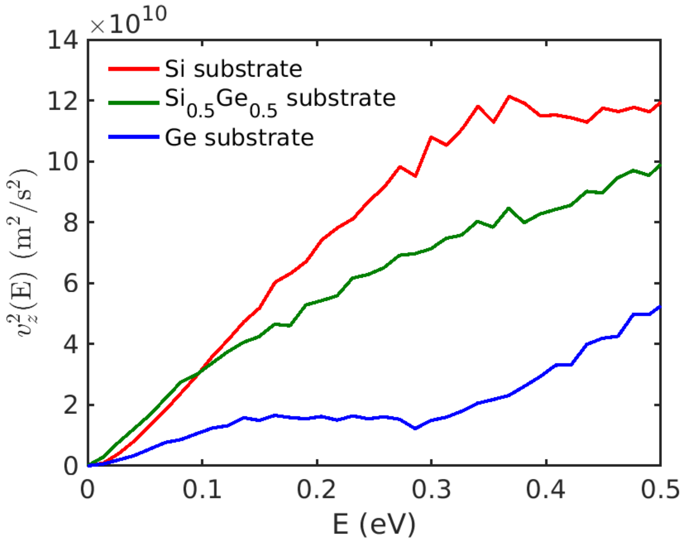


Figure 8: Squared electronic group velocity in strained $Si_2Ge_2$ SLs along the cross-plane ($z$) direction. The red, green and blue lines represent $Si_2Ge_2$ SLs assumed to be grown on Si, $Si_{0.5}Ge_{0.5}$, and Ge substrates, respectively.

## Resistivity Predictions of $Si_2Ge_2$ SLs Grown on Varying Substrates using CRTA

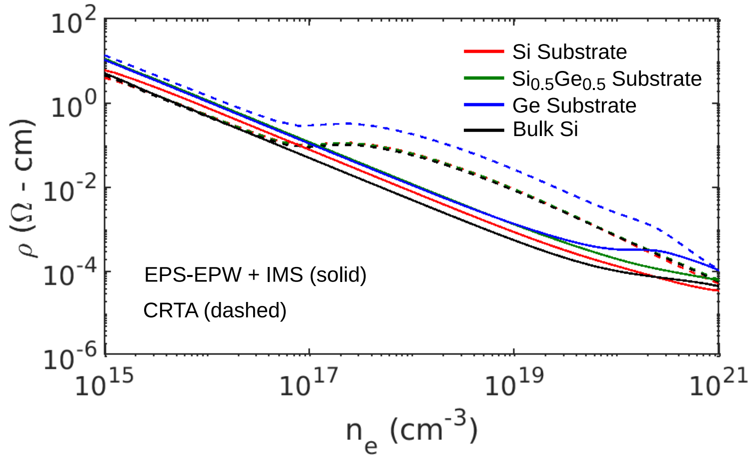


Figure 9: Comparison between predicted cross-plane resistivity of strained $Si_2Ge_2$ SLs, using the constant relaxation time approximation (CRTA) (dashed lines) and relaxation times due to EPS-EPW+IMS processes (solid lines). The red, green and blue lines represent $Si_2Ge_2$ SLs assumed to be grown on Si, $Si_{0.5}Ge_{0.5}$, and Ge substrates, respectively. $\tau$ values are extracted from measured bulk Si mobility data[4] to obtain the CRTA predictions. The CRTA is particularly inaccurate at the high doping regime.

# References


(1) Semiconductor, V. *General Properties of Si, Ge, SiGe, SiO2 and Si3N4*; 2002.

(2) Ashcroft, N. W.; Mermin, N. D. *Solid State Physics*; Saunders, Philadelphia, 1976.

(3) Hummer, K.; Harl, J.; Kresse, G. Heyd-Scuseria-Ernzerhof hybrid functional for calculating the lattice dynamics of semiconductors. *Physical Review B* **2009**, *80*, 115205.

(4) Jacoboni, C.; Canali, C.; Ottaviani, G.; Quaranta, A. A. A review of some charge transport properties of silicon. *Solid-State Electronics* **1977**, *20*, 77–89.
